# Supplementary material for: Prospects of forming high-spin polar molecules from ultracold atoms
Source: arXiv:1910.09641 ancillary file (2020-07-30)
Supplement: Supplementary file 1 [file Dy_Yb_supp.pdf]

# Supplemental Material for Prospects of forming high-spin polar molecules from ultracold atoms

Matthew D. Frye,<sup>1</sup> Simon L. Cornish,<sup>2</sup> and Jeremy M. Hutson<sup>1,\*</sup>

<sup>1</sup>*Joint Quantum Centre (JQC) Durham-Newcastle, Department of Chemistry,  
Durham University, South Road, Durham, DH1 3LE, United Kingdom.*

<sup>2</sup>*Joint Quantum Centre (JQC) Durham-Newcastle, Department of Physics,  
Durham University, South Road, Durham, DH1 3LE, United Kingdom.*

(Dated: March 17, 2020)

---

\* j.m.hutson@durham.ac.uk

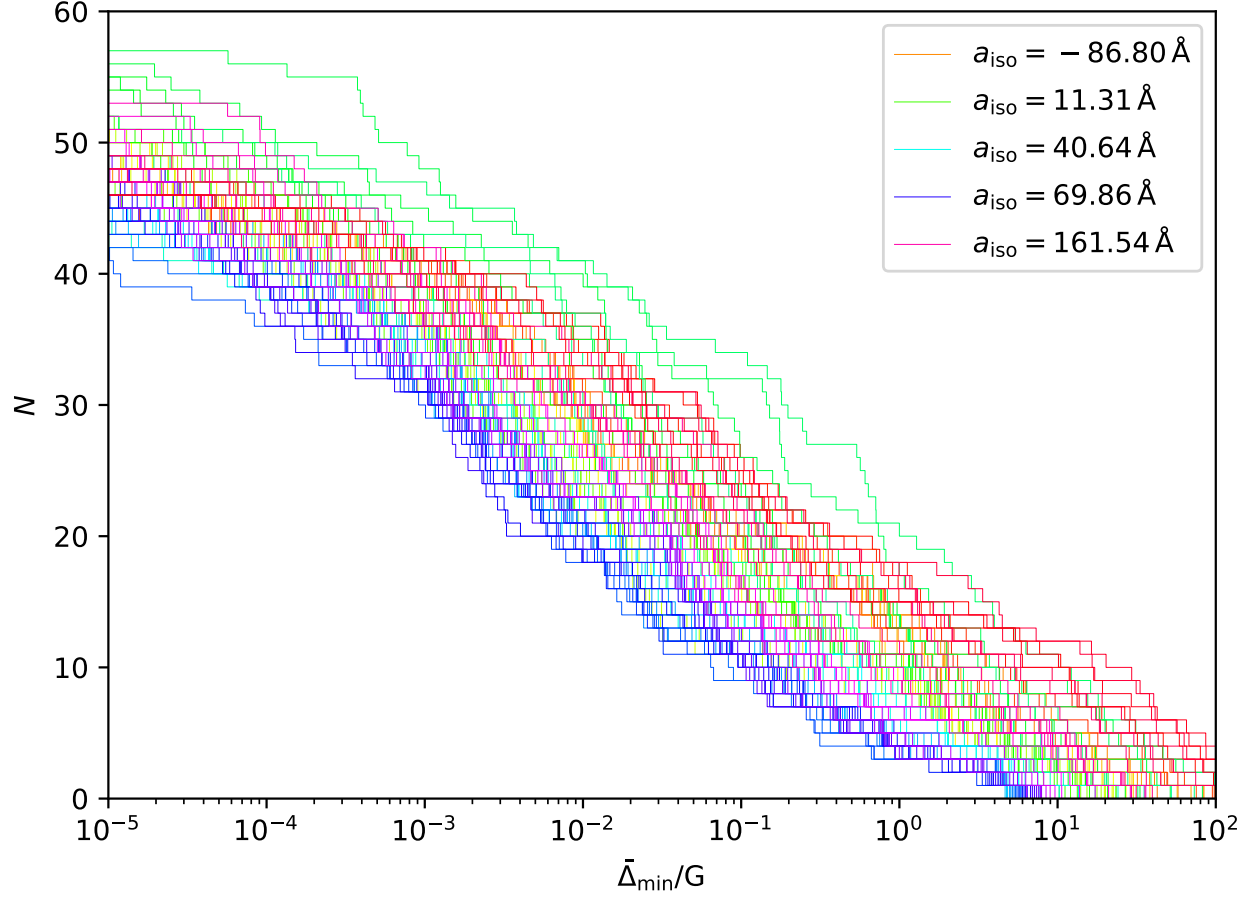

FIG. 1. Number of resonances below 500 G with normalised widths  $\bar{\Delta}$  greater than  $\bar{\Delta}_{\min}$  for 100 potentials for Dy+Yb with long-range anisotropy  $C_6^{(2)}/C_6^{(0)} = 0.017$ .

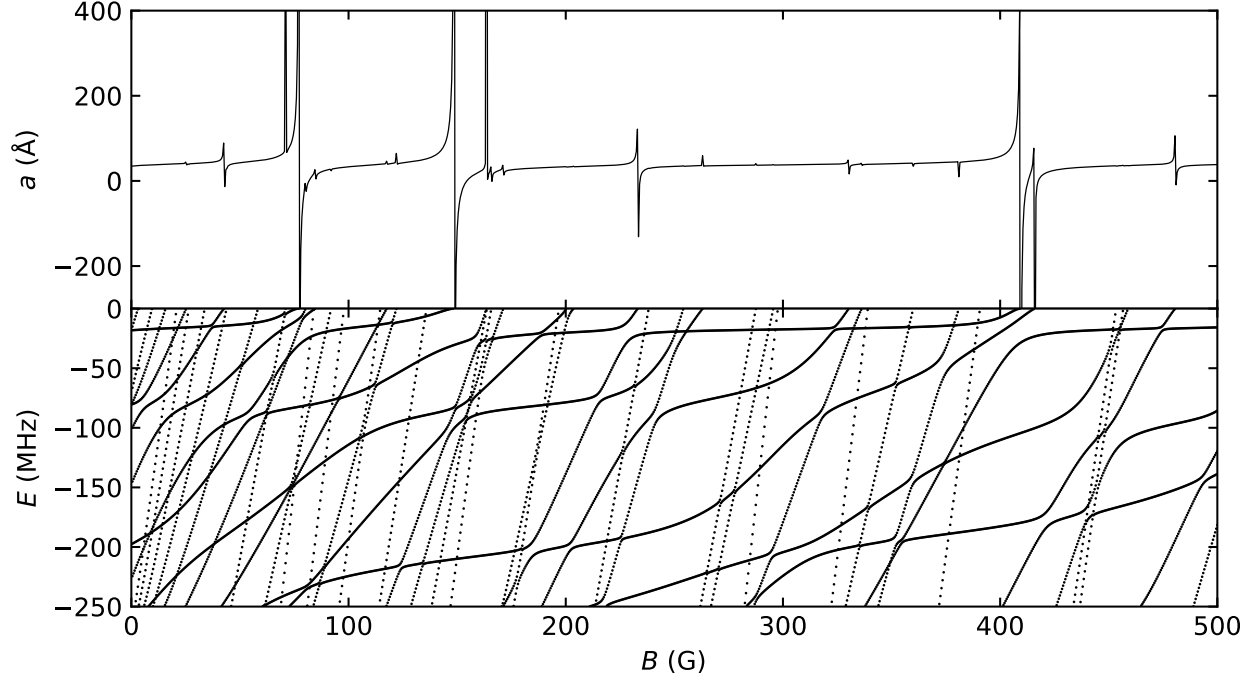

FIG. 2. Scattering lengths as a function of magnetic field for Dy+Yb with long-range anisotropy  $C_6^{(2)}/C_6^{(0)} = 0.017$  for  $a_{\text{iso}} = 54$  Å. Bottom: The corresponding near-threshold bound states.

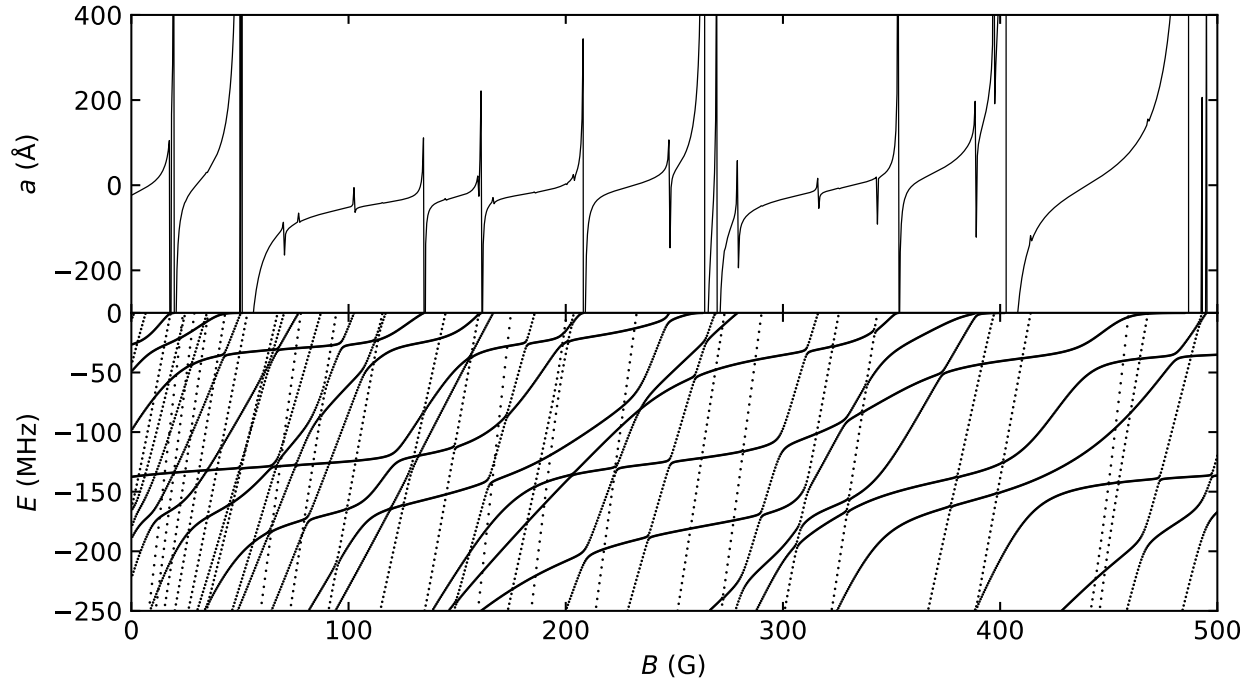

FIG. 3. Scattering lengths as a function of magnetic field for Dy+Yb with long-range anisotropy  $C_6^{(2)}/C_6^{(0)} = 0.017$  for  $a_{\text{iso}} = -80$  Å. Bottom: The corresponding near-threshold bound states.

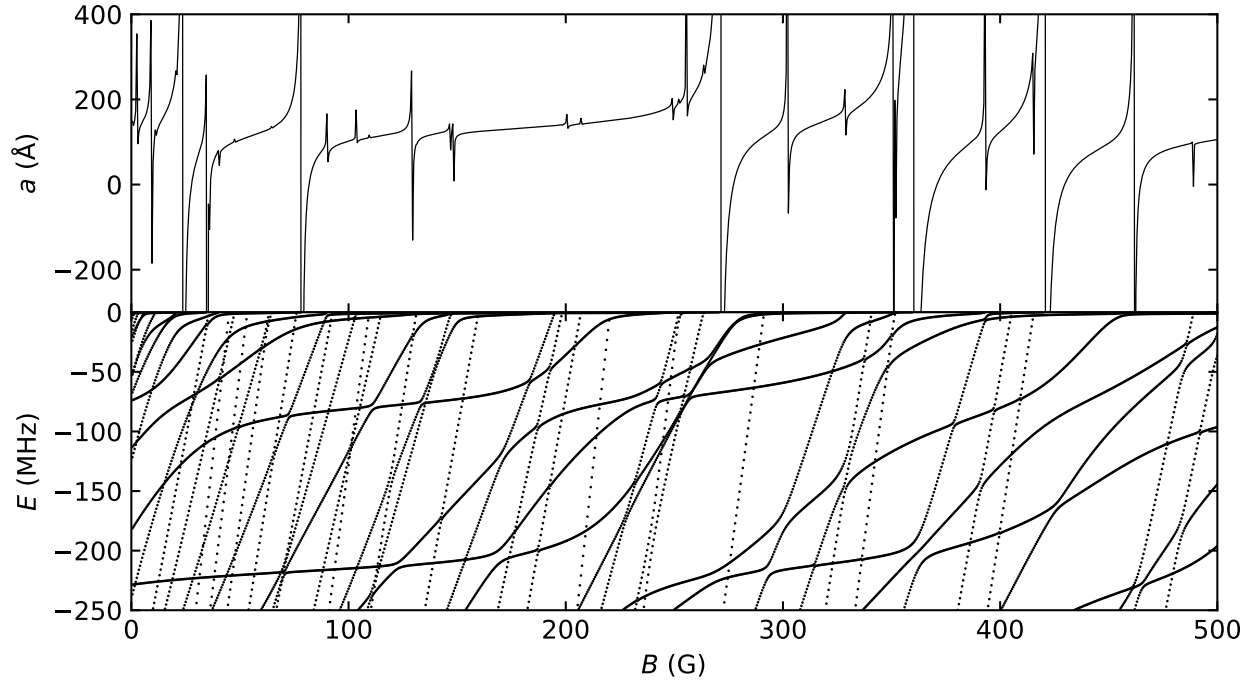

FIG. 4. Scattering lengths as a function of magnetic field for Dy+Yb with long-range anisotropy  $C_6^{(2)}/C_6^{(0)} = 0.017$  for  $a_{\text{iso}} = 168$  Å. Bottom: The corresponding near-threshold bound states.

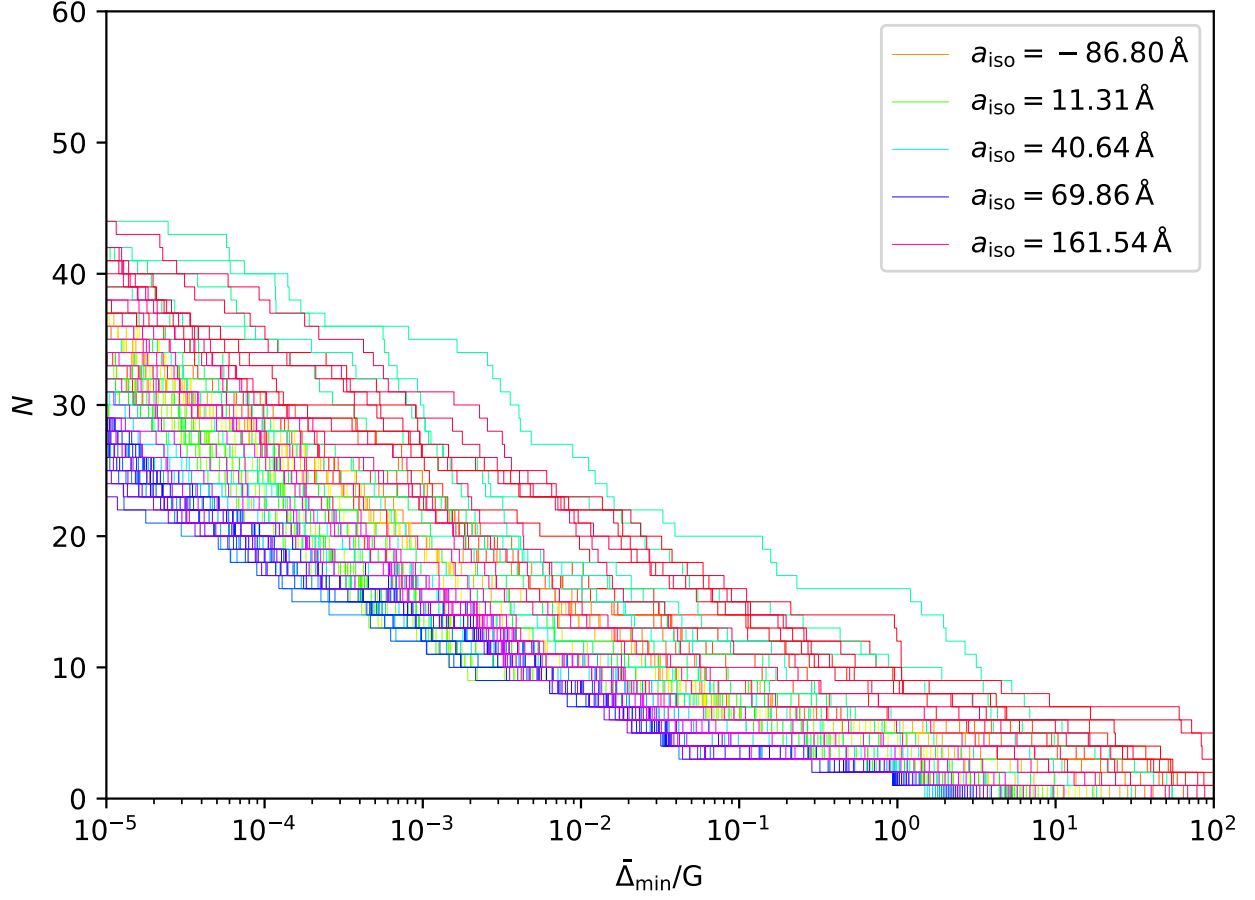

FIG. 5. Number of resonances below 500 G with normalised widths  $\bar{\Delta}$  greater than  $\bar{\Delta}_{\min}$  for 100 potentials for Dy+Yb with long-range anisotropy  $C_6^{(2)}/C_6^{(0)} = 0.0085$ .

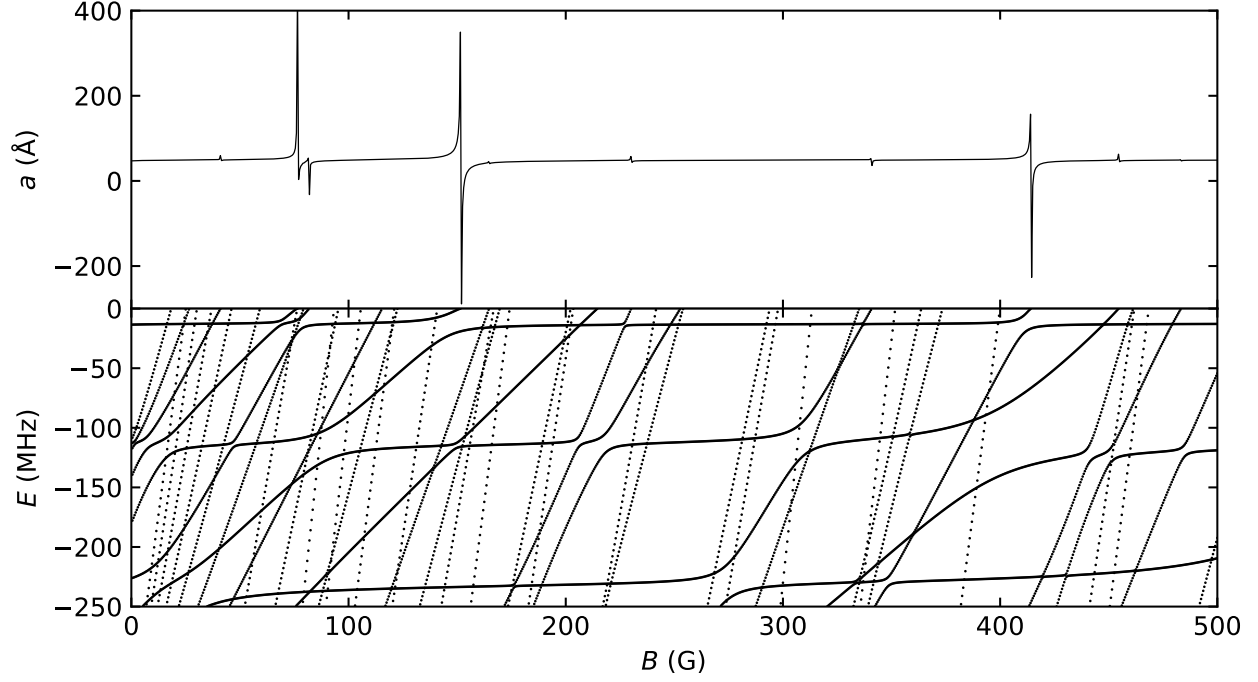

FIG. 6. Scattering lengths as a function of magnetic field for Dy+Yb with long-range anisotropy  $C_6^{(2)}/C_6^{(0)} = 0.0085$  for  $a_{\text{iso}} = 54$  Å. Bottom: The corresponding near-threshold bound states.

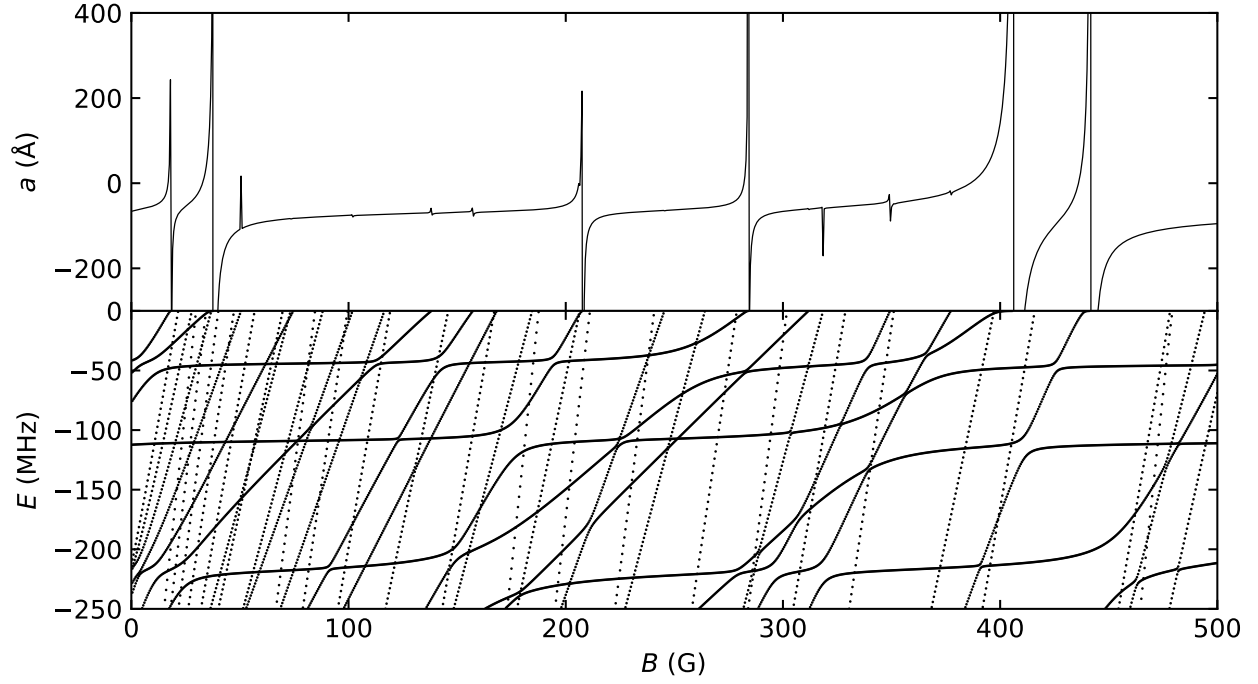

FIG. 7. Scattering lengths as a function of magnetic field for Dy+Yb with long-range anisotropy  $C_6^{(2)}/C_6^{(0)} = 0.0085$  for  $a_{\text{iso}} = -80$  Å. Bottom: The corresponding near-threshold bound states.

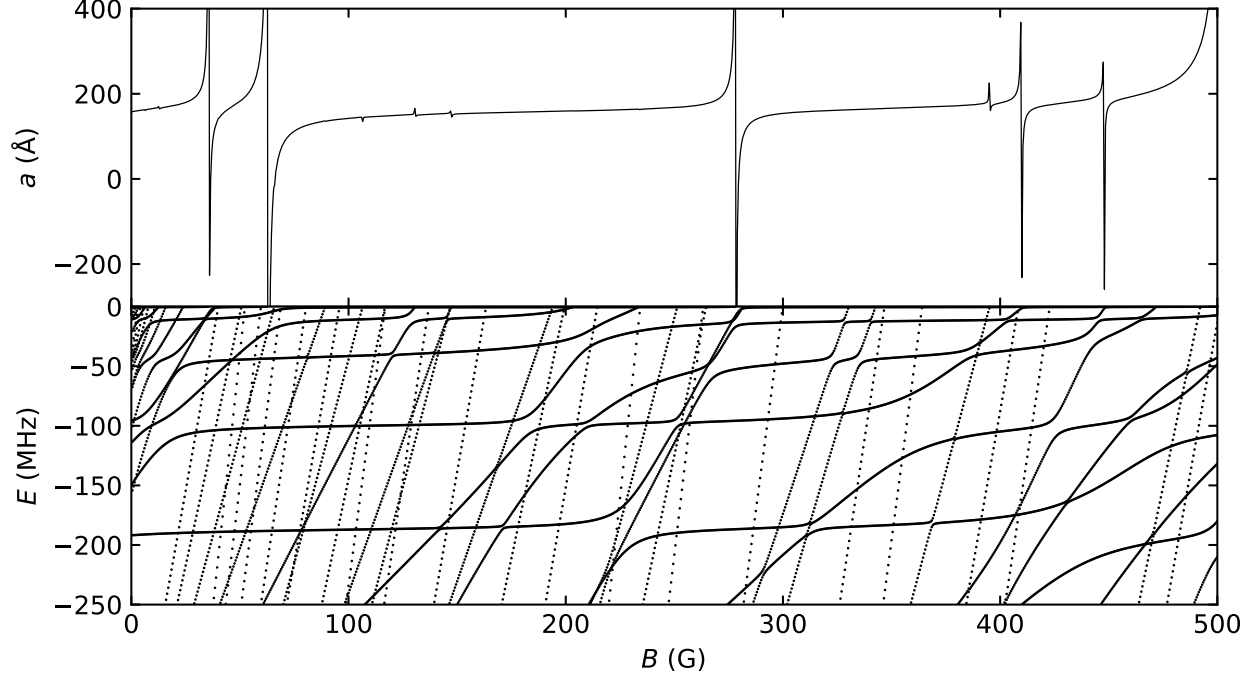

FIG. 8. Scattering lengths as a function of magnetic field for Dy+Yb with long-range anisotropy  $C_6^{(2)}/C_6^{(0)} = 0.0085$  for  $a_{\text{iso}} = 168$  Å. Bottom: The corresponding near-threshold bound states.

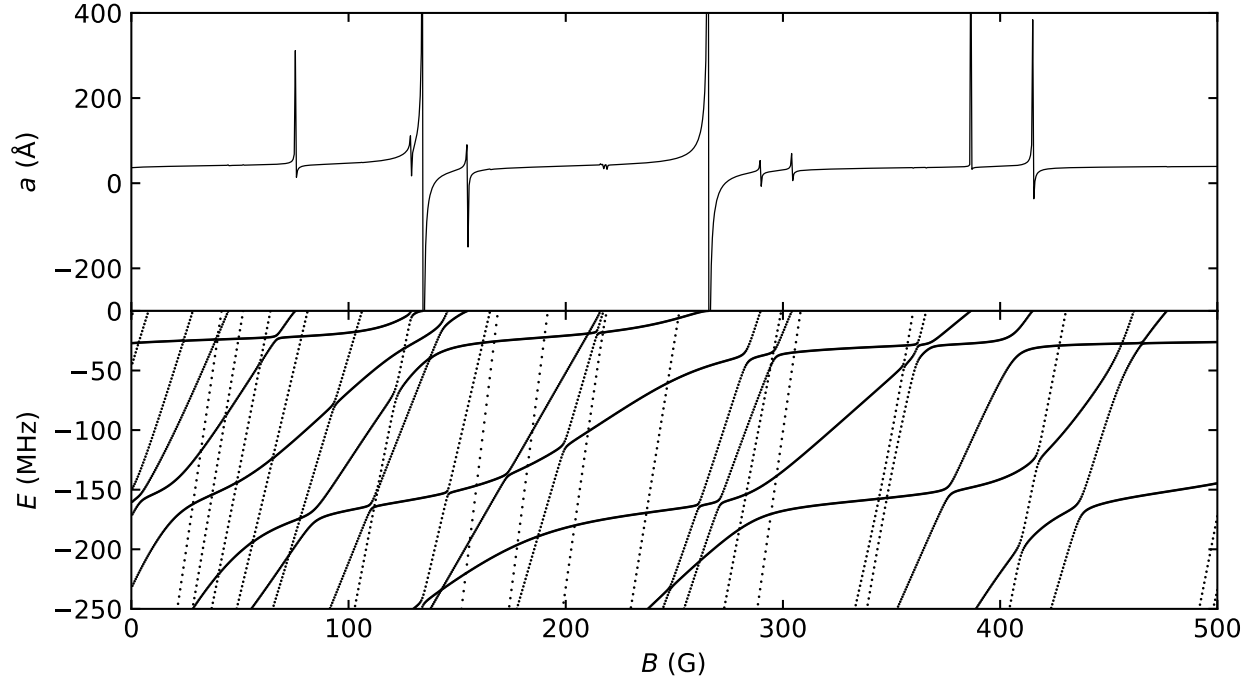

FIG. 9. Scattering lengths as a function of magnetic field for Er+Sr with long-range anisotropy  $C_6^{(2)}/C_6^{(0)} = 0.017$  for  $a_{\text{iso}} = 51$  Å. Bottom: The corresponding near-threshold bound states.

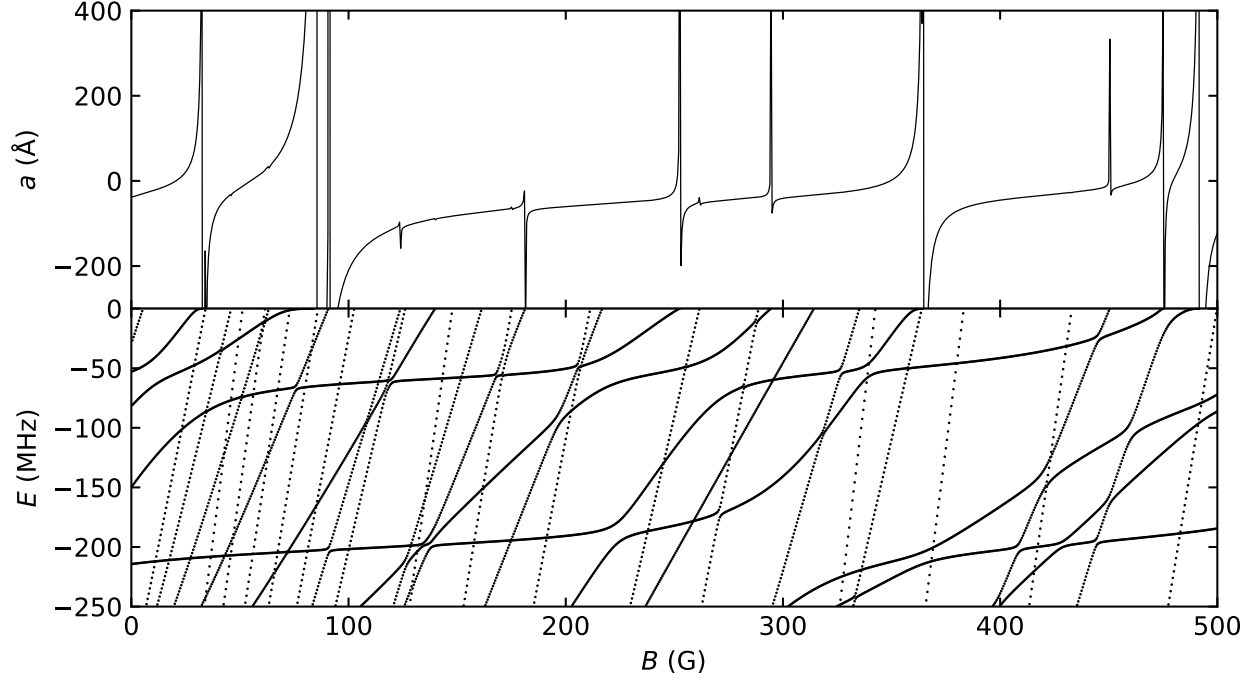

FIG. 10. Scattering lengths as a function of magnetic field for Er+Sr with long-range anisotropy  $C_6^{(2)}/C_6^{(0)} = 0.017$  for  $a_{\text{iso}} = -74$  Å. Bottom: The corresponding near-threshold bound states.

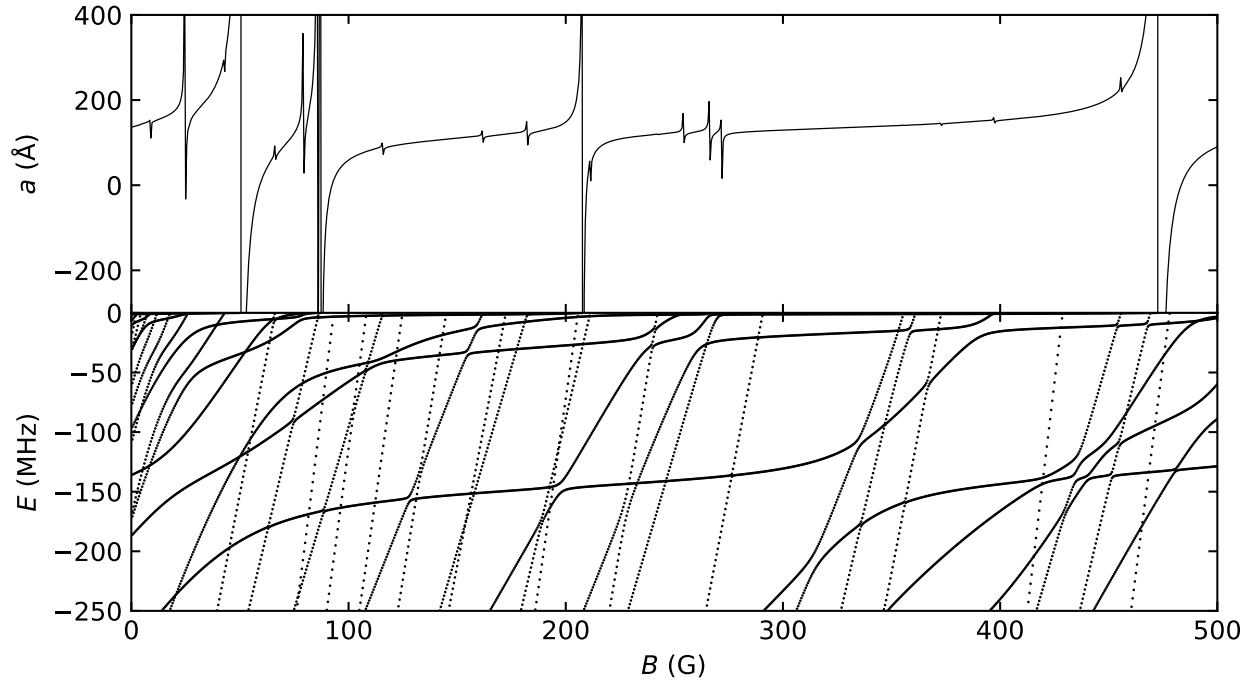

FIG. 11. Scattering lengths as a function of magnetic field for Er+Sr with long-range anisotropy  $C_6^{(2)}/C_6^{(0)} = 0.017$  for  $a_{\text{iso}} = 158$  Å. Bottom: The corresponding near-threshold bound states.



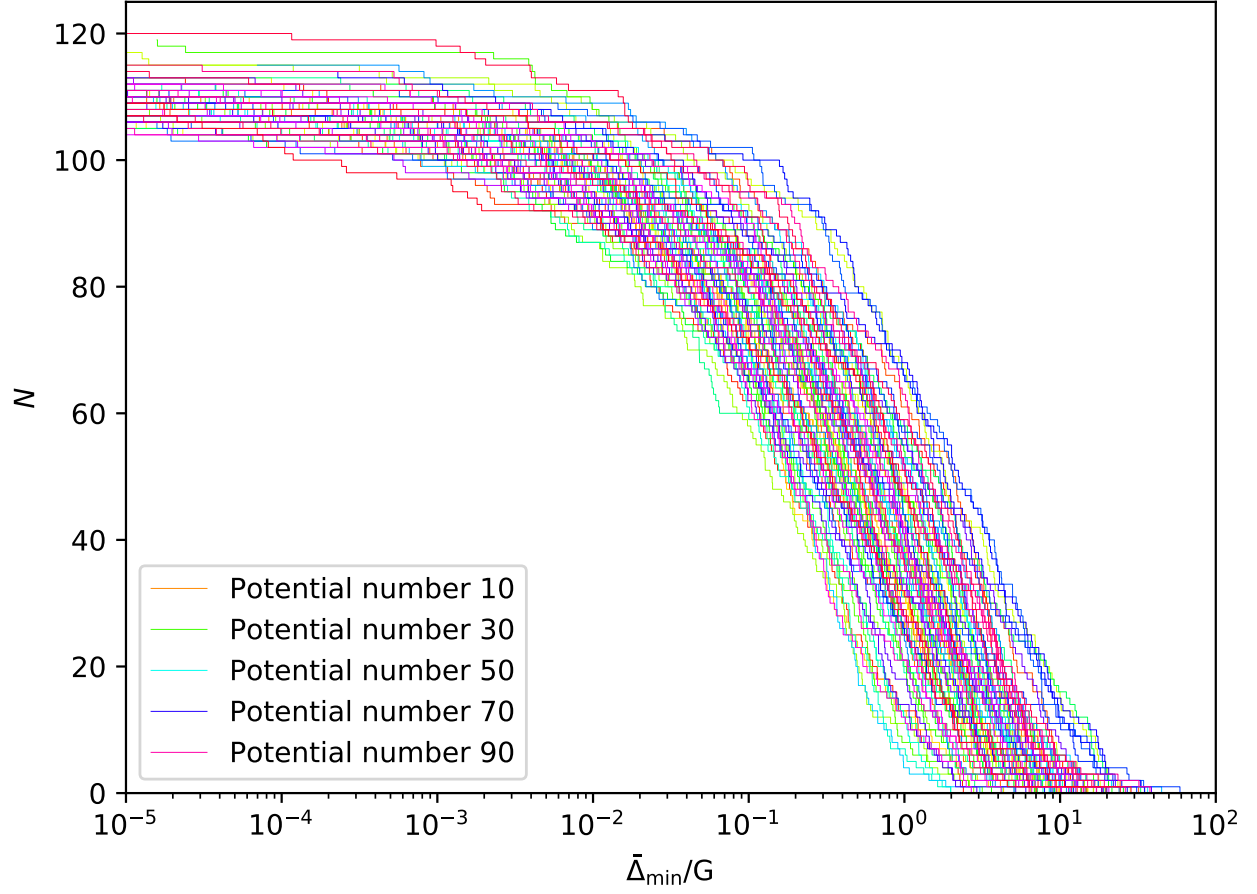

FIG. 12. Number of resonances below 500 G with normalised widths  $\bar{\Delta}$  greater than  $\bar{\Delta}_{\min}$  for 100 potentials for Dy+Yb with short-range anisotropy as described in the main text.

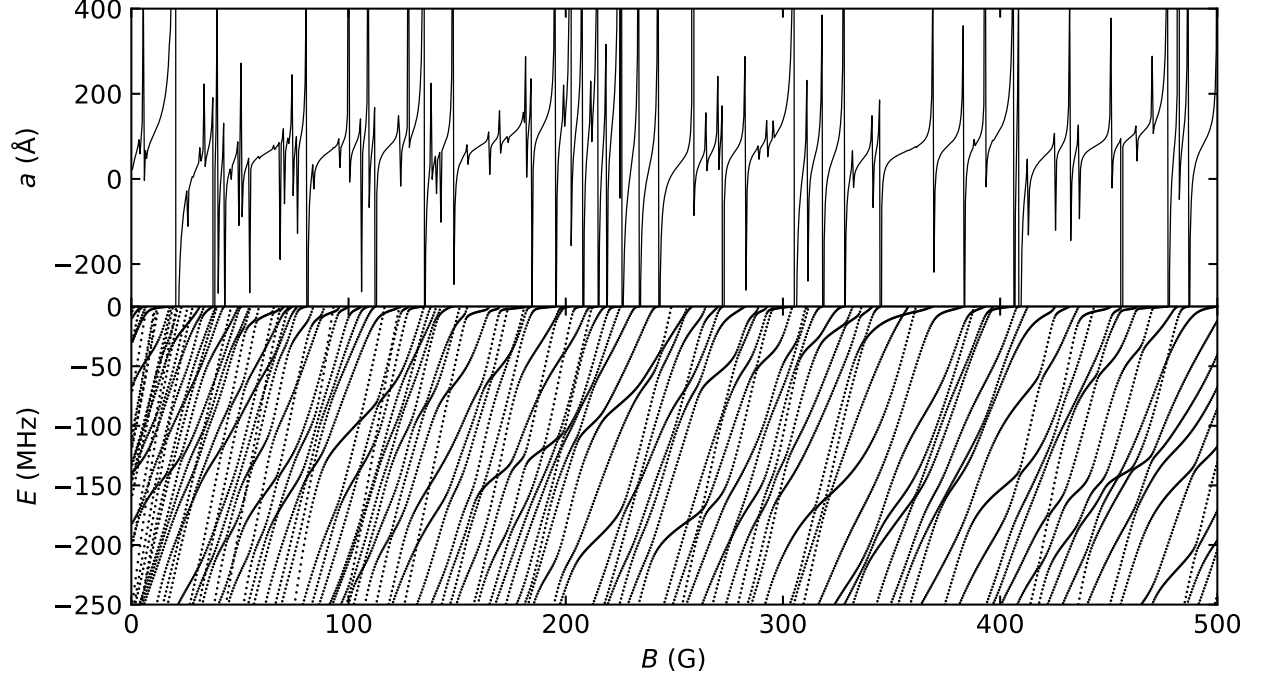

FIG. 13. Top: Scattering lengths as a function of field for Dy+Yb with short-range anisotropy as described in the main text. Bottom: The corresponding near-threshold bound states. First example.

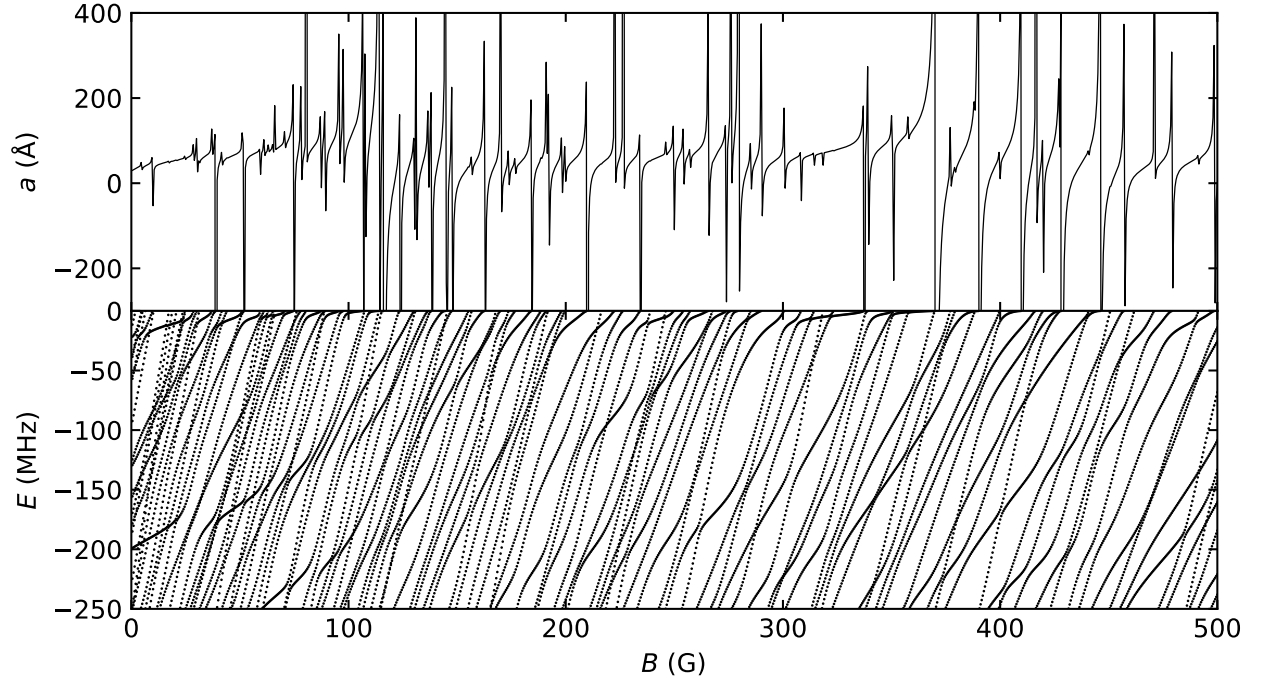

FIG. 14. Top: Scattering lengths as a function of field for Dy+Yb with short-range anisotropy as described in the main text. Bottom: The corresponding near-threshold bound states. Second example.

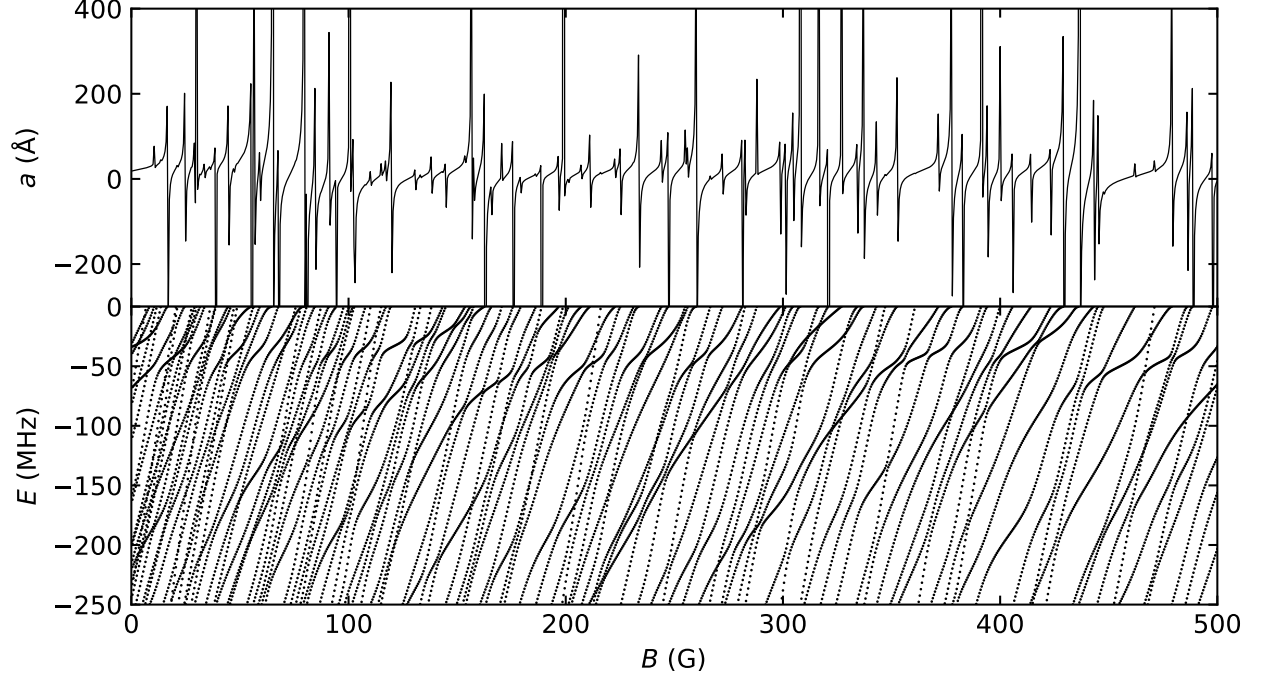

FIG. 15. Top: Scattering lengths as a function of field for Dy+Yb with short-range anisotropy as described in the main text. Bottom: The corresponding near-threshold bound states. Third example.

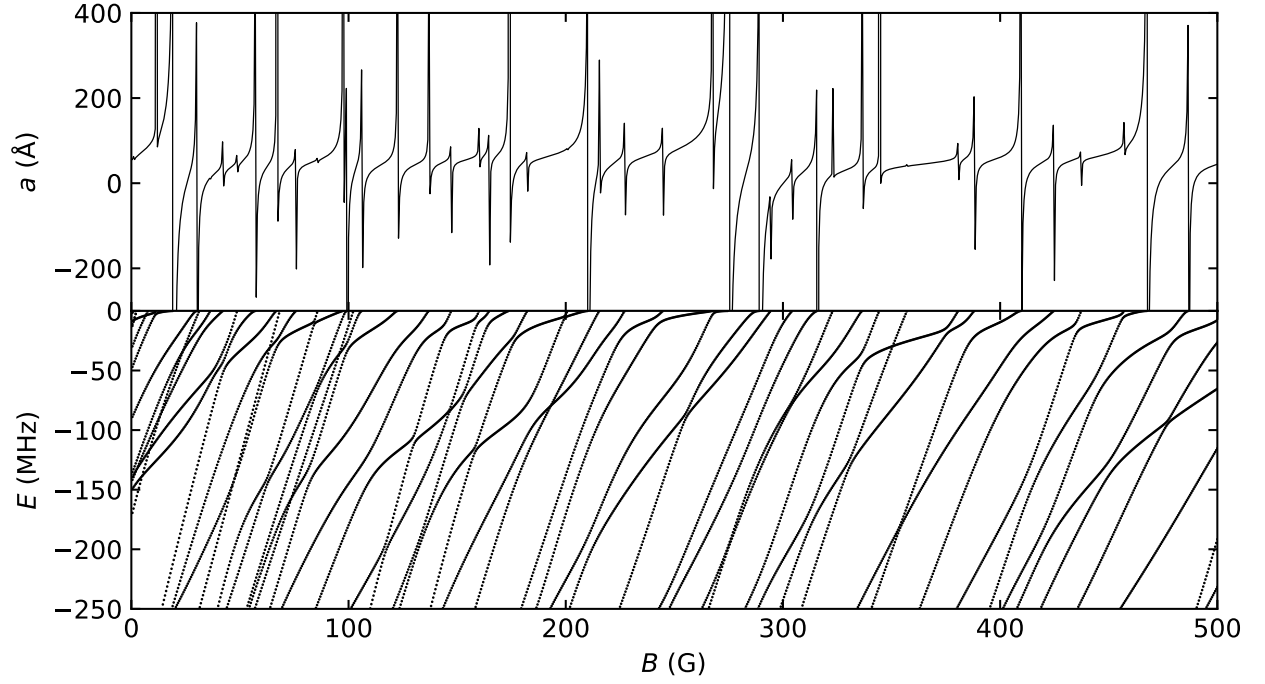

FIG. 16. Top: Scattering lengths as a function of field for Er+Sr with short-range anisotropy as described in the main text. Bottom: The corresponding near-threshold bound states. First example.

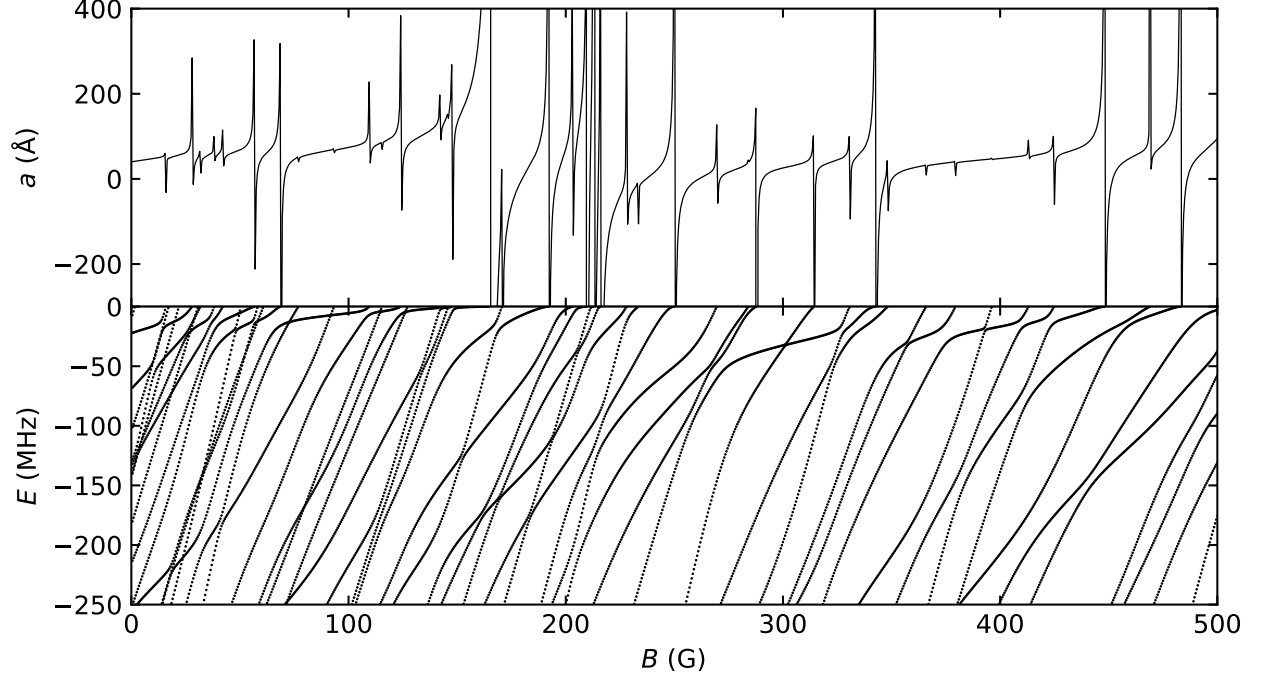

FIG. 17. Top: Scattering lengths as a function of field for Er+Sr with short-range anisotropy as described in the main text. Bottom: The corresponding near-threshold bound states. Second example.

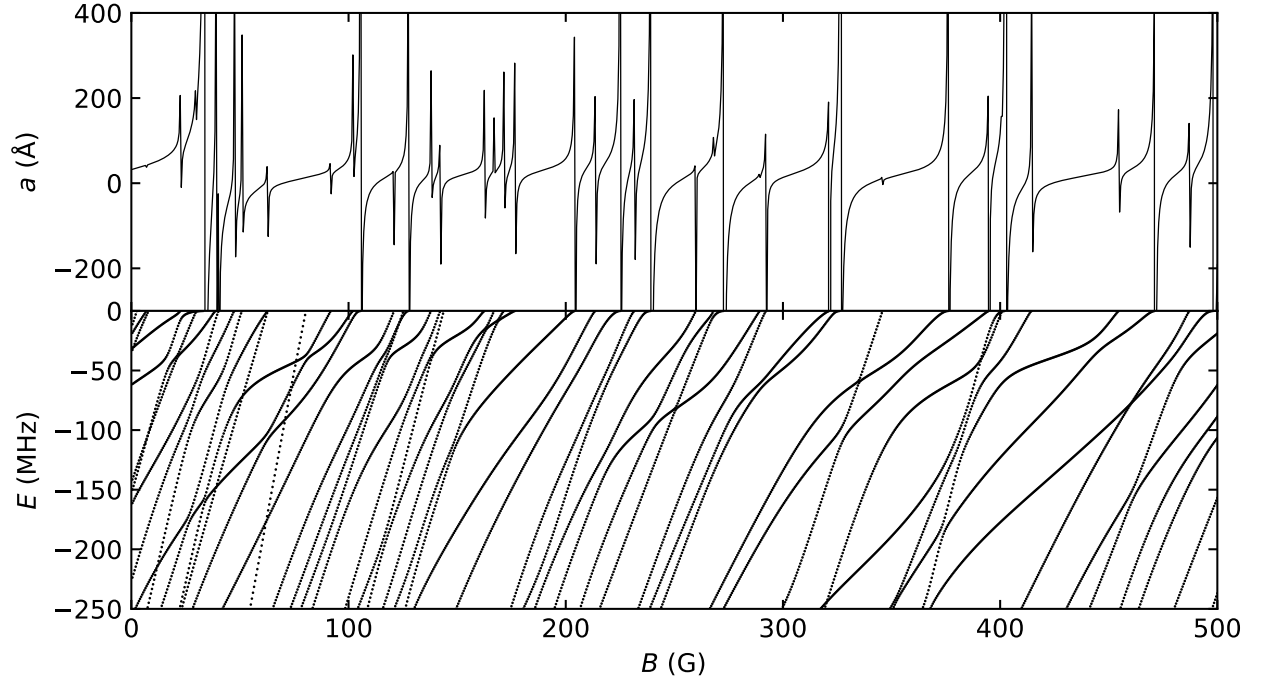

FIG. 18. Top: Scattering lengths as a function of field for Er+Sr with short-range anisotropy as described in the main text. Bottom: The corresponding near-threshold bound states. Third example.



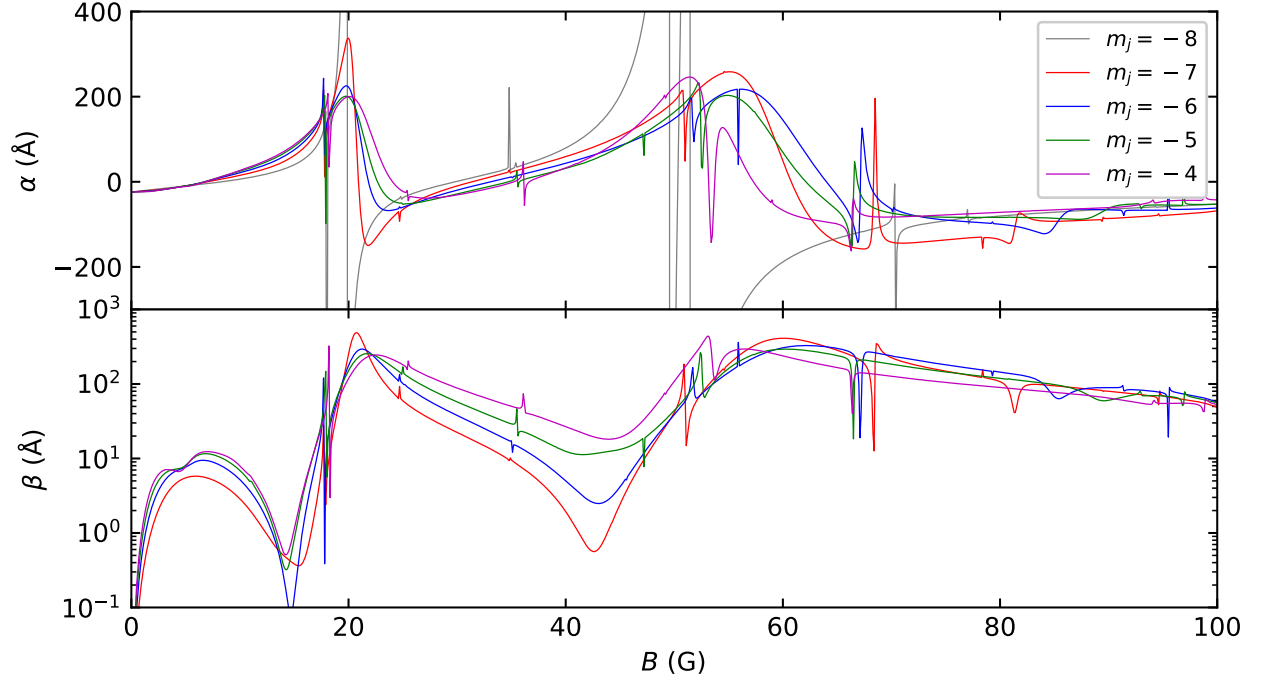

FIG. 19. Complex scattering lengths  $a = \alpha - i\beta$  as a function of magnetic field for Dy+Yb with Dy in excited Zeeman states  $m_j = -7$  (red),  $-6$  (blue),  $-5$  (green), and  $-4$  (magenta);  $m_j = -8$  (grey) results are also shown for comparison. Interaction potential with long-range anisotropy  $C_6^{(2)}/C_6^{(0)} = 0.017$  for  $a_{\text{iso}} = -80$  Å.

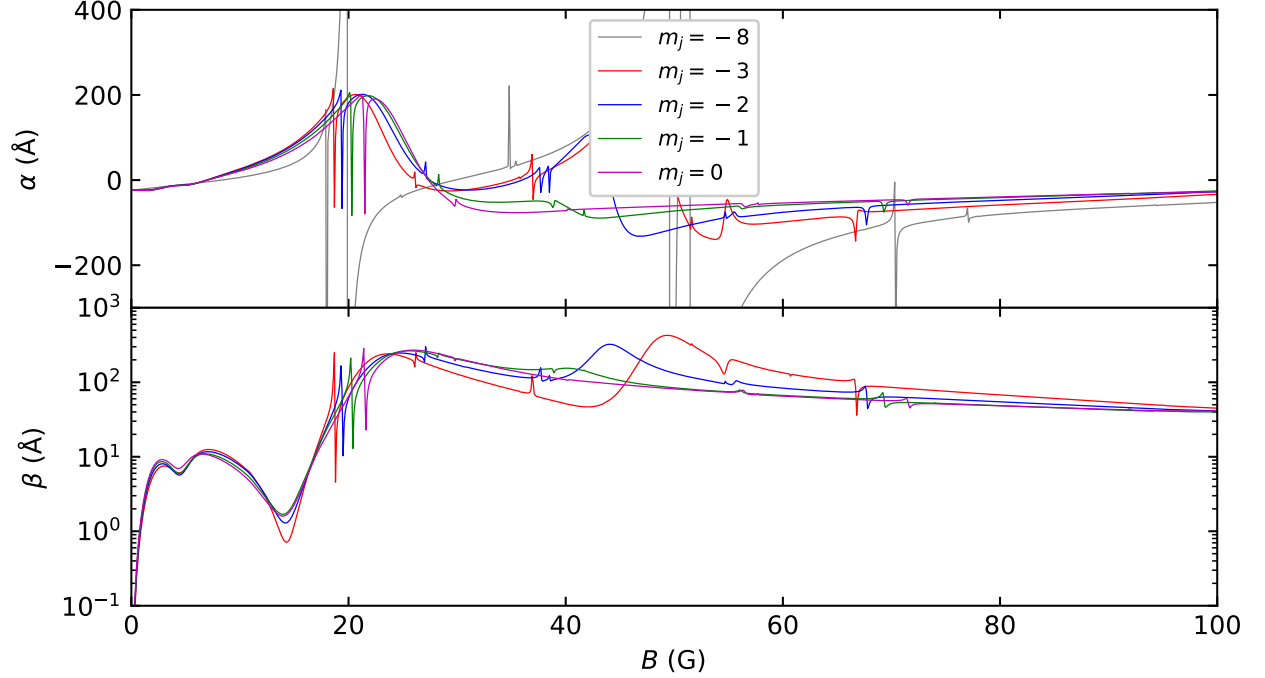

FIG. 20. Complex scattering lengths  $a = \alpha - i\beta$  as a function of magnetic field for Dy+Yb with Dy in excited Zeeman states  $m_j = -3$  (red),  $-2$  (blue),  $-1$  (green), and  $0$  (magenta);  $m_j = -8$  (grey) results are also shown for comparison. Interaction potential with long-range anisotropy  $C_6^{(2)}/C_6^{(0)} = 0.017$  for  $a_{\text{iso}} = -80$  Å.

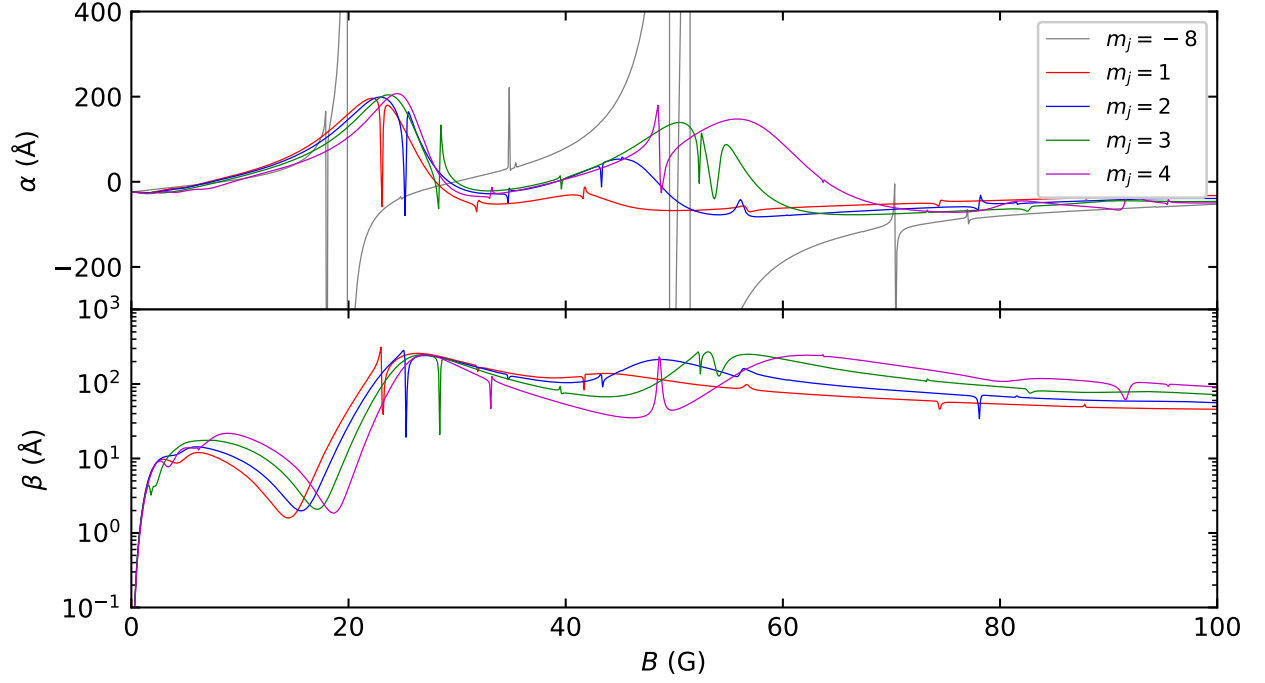

FIG. 21. Complex scattering lengths  $a = \alpha - i\beta$  as a function of magnetic field for Dy+Yb with Dy in excited Zeeman states  $m_j = 1$  (red), 2 (blue), 3 (green), and 4 (magenta);  $m_j = -8$  (grey) results are also shown for comparison. Interaction potential with long-range anisotropy  $C_6^{(2)}/C_6^{(0)} = 0.017$  for  $a_{\text{iso}} = -80$  Å.

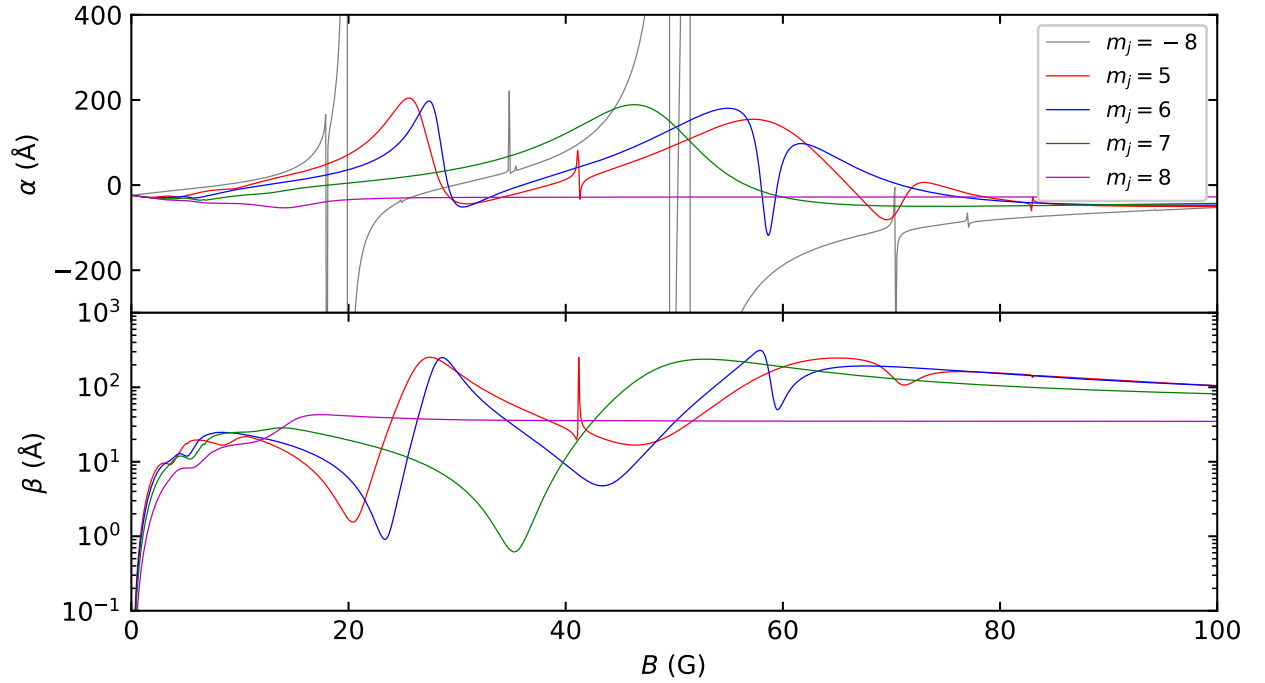

FIG. 22. Complex scattering lengths  $a = \alpha - i\beta$  as a function of magnetic field for Dy+Yb with Dy in excited Zeeman states  $m_j = 5$  (red), 6 (blue), 7 (green), and 8 (magenta);  $m_j = -8$  (grey) results are also shown for comparison. Interaction potential with long-range anisotropy  $C_6^{(2)}/C_6^{(0)} = 0.017$  for  $a_{\text{iso}} = -80$  Å.

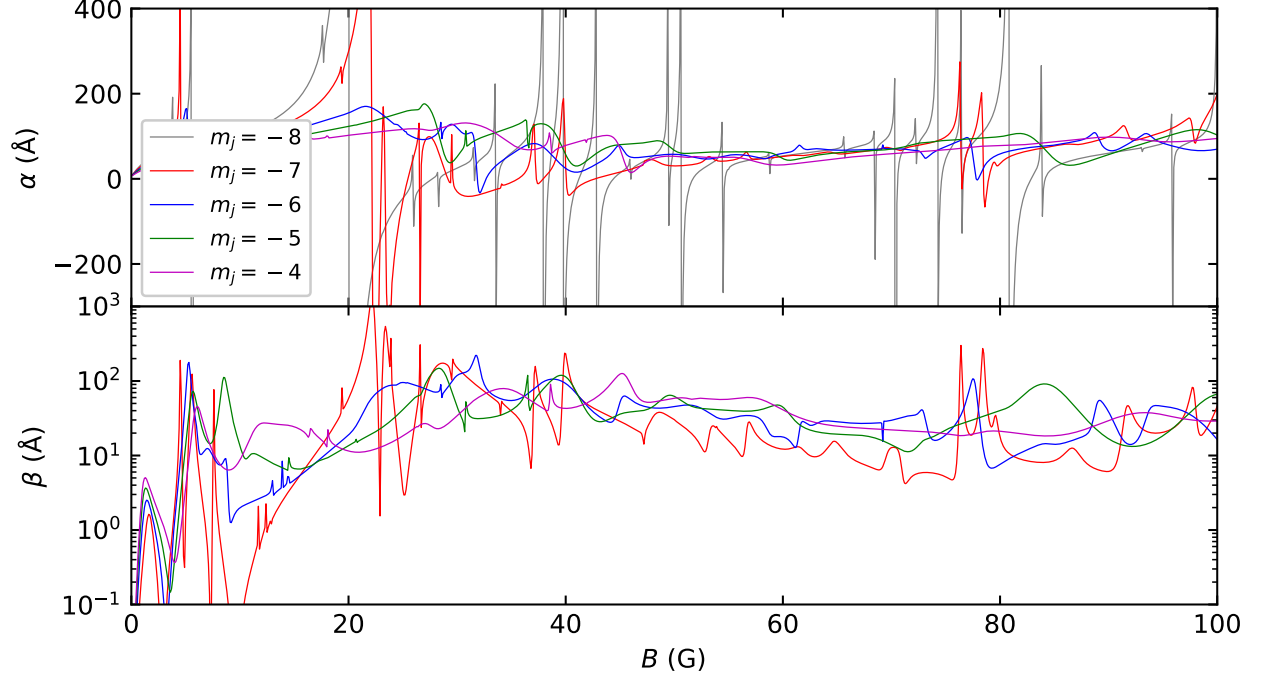

FIG. 23. Complex scattering lengths  $a = \alpha - i\beta$  as a function of magnetic field for Dy+Yb with Dy in excited Zeeman states  $m_j = -7$  (red),  $-6$  (blue),  $-5$  (green), and  $-4$  (magenta);  $m_j = -8$  (grey) results are also shown for comparison. Interaction potential with short-range anisotropy as described in the main text.

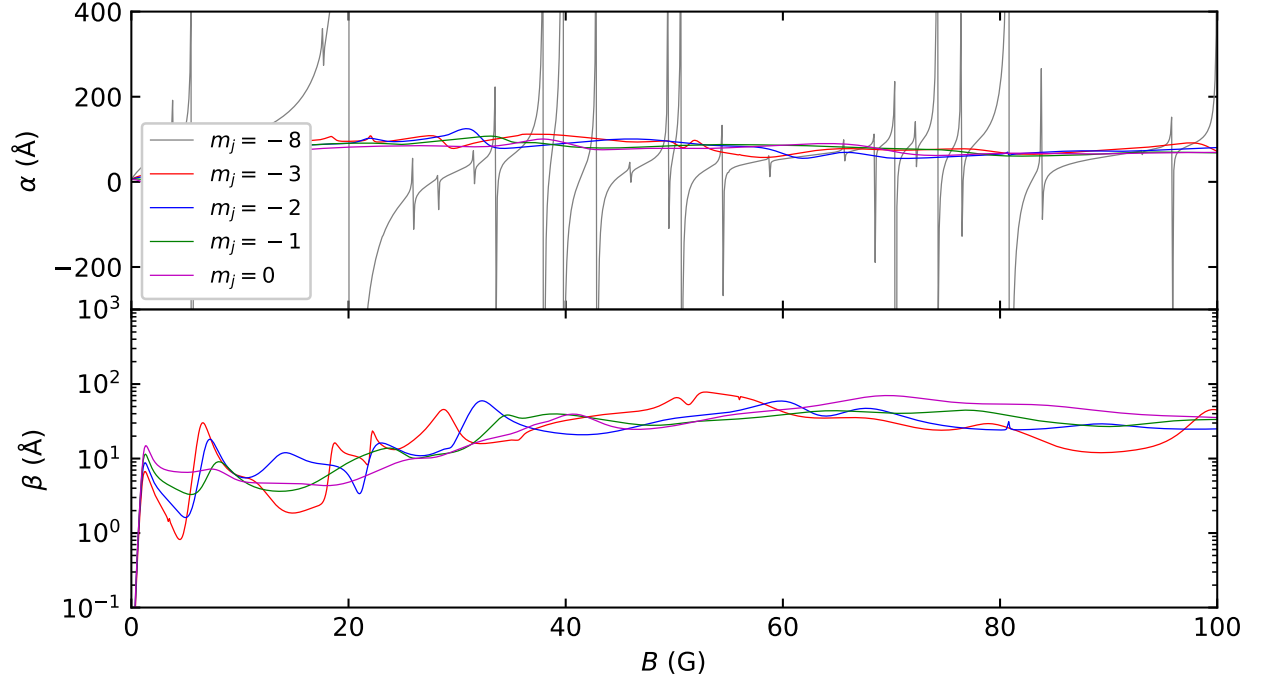

FIG. 24. Complex scattering lengths  $a = \alpha - i\beta$  as a function of magnetic field for Dy+Yb with Dy in excited Zeeman states  $m_j = -3$  (red),  $-2$  (blue),  $-1$  (green), and  $0$  (magenta);  $m_j = -8$  (grey) results are also shown for comparison. Interaction potential with short-range anisotropy as described in the main text.



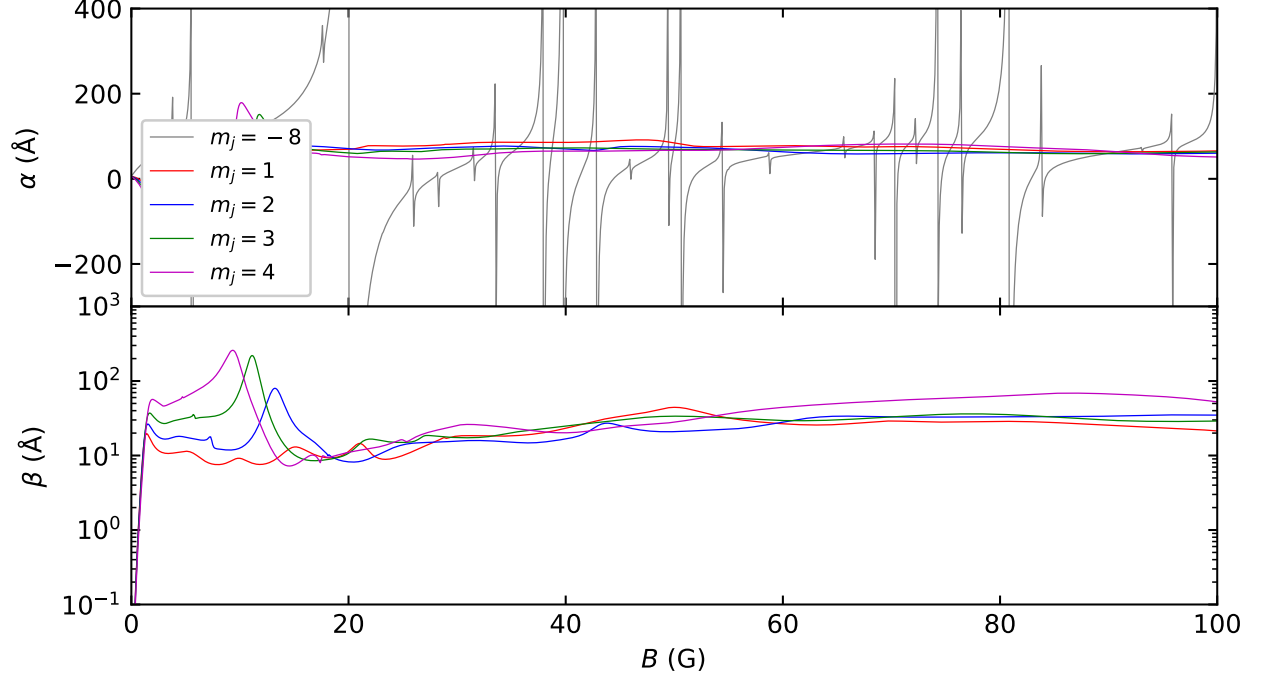

FIG. 25. Complex scattering lengths  $a = \alpha - i\beta$  as a function of magnetic field for Dy+Yb with Dy in excited Zeeman states  $m_j = 1$  (red), 2 (blue), 3 (green), and 4 (magenta);  $m_j = -8$  (grey) results are also shown for comparison. Interaction potential with short-range anisotropy as described in the main text.

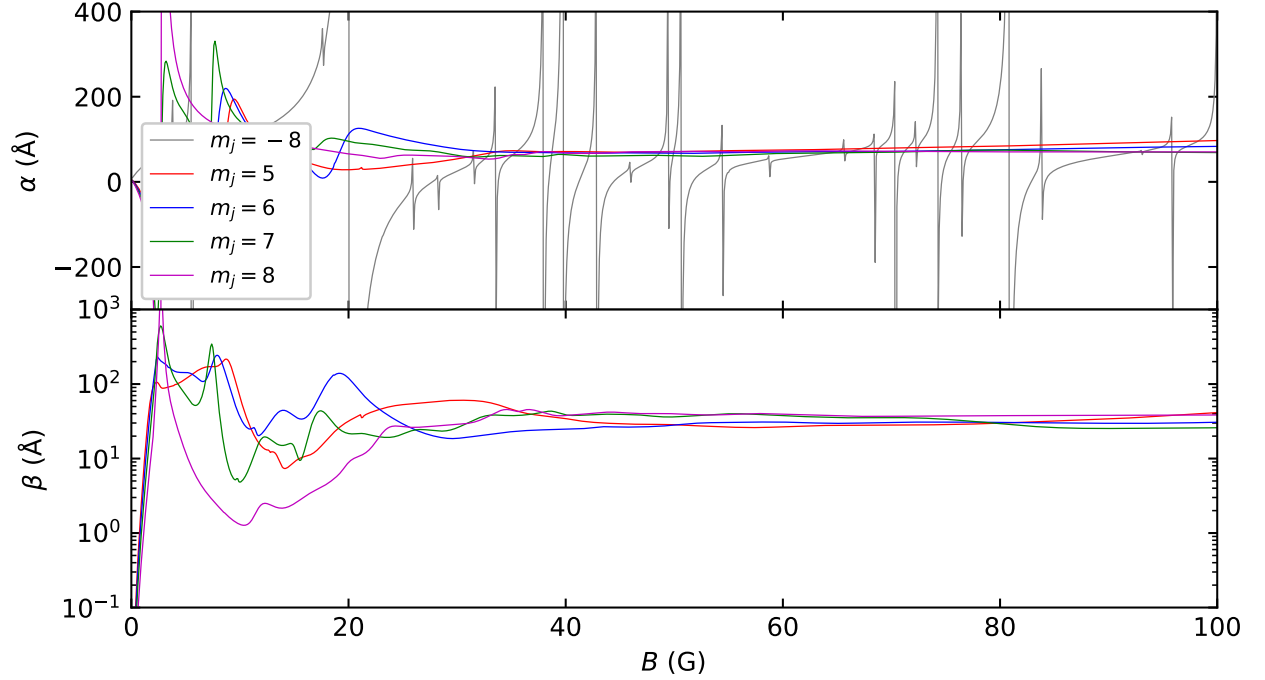

FIG. 26. Complex scattering lengths  $a = \alpha - i\beta$  as a function of magnetic field for Dy+Yb with Dy in excited Zeeman states  $m_j = 5$  (red), 6 (blue), 7 (green), and 8 (magenta);  $m_j = -8$  (grey) results are also shown for comparison. Interaction potential with short-range anisotropy as described in the main text.
